# Supplementary material for: Harmonizing knowledge Transfer in Neural Network with Unified Distillation
Source: arXiv:2409.18565 source file (2024-09-27)
Supplement: Supplementary file 1 [file X_suppl.tex]

\clearpage
\setcounter{page}{1}
\begin{center}
\textbf{\Large Supplementary Materials for \\
Harmonizing knowledge Transfer in Neural Network with Unified Distillation}
\end{center}
% \maketitlesupplementary

\setcounter{section}{0}
This supplementary material further validates our distillation approach by extending its application from CNNs to ViTs, and offering a detailed explanation of the experimental settings.

\section{The Analytical Solution to the KL Divergence of Multivariate Gaussian Distributions}
if $p(x)=\mathcal{N}\left(\mu_1, \Sigma_1\right), q(x)=\mathcal{N}\left(\mu_2, \Sigma_2\right)$ , then:
$$
\begin{aligned}
& D_{K L}\left[\mathcal{N}\left(\mu_1, \Sigma_1\right) \| \mathcal{N}\left(\mu_2, \Sigma_2\right)\right] \\
& =D_{K L}[p(x) \| q(x)] \\
& =\int p(x) \log \frac{p(x)}{q(x)} \\
& =E_{p(x)}[\log p(x)-\log q(x)] \\
& =E_{p(x)}[\log \left\{\frac{1}{(2 \pi)^{d / 2}\left|\Sigma_1\right|^{1 / 2}} \exp \left[-\frac{1}{2}\left(x-\mu_1\right)^{\mathcal{T}} \Sigma_1^{-1}\left(x-\mu_1\right)\right]\right\} \\
& -\log \left\{\frac{1}{(2 \pi)^{d / 2}\left|\Sigma_2\right|^{1 / 2}} \exp \left[-\frac{1}{2}\left(x-\mu_2\right)^{\mathcal{T}} \Sigma_2^{-1}\left(x-\mu_2\right)\right]\right\}] \\
& =E_{p(x)}[\log \frac{1}{(2 \pi)^{d / 2}}+\log \frac{1}{\left|\Sigma_1\right|^{1 / 2}}-\frac{1}{2}\left(x-\mu_1\right)^{\mathcal{T}} \Sigma_1^{-1}\left(x-\mu_1\right) \\
& - \left\{\log \frac{1}{(2 \pi)^{d / 2}}+\log \frac{1}{\left|\Sigma_2\right|^{1 / 2}}-\frac{1}{2}\left(x-\mu_2\right)^{\mathcal{T}} \Sigma_2^{-1}\left(x-\mu_2\right)\right\}] \\
& =E_{p(x)}\left[\log \frac{\left|\Sigma_2\right|^{1 / 2}}{\left|\Sigma_1\right|^{1 / 2}}-\frac{1}{2}\left(x-\mu_1\right)^{\mathcal{T}} \Sigma_1^{-1}\left(x-\mu_1\right)+\frac{1}{2}\left(x-\mu_2\right)^{\mathcal{T}} \Sigma_2^{-1}\left(x-\mu_2\right)\right] \\
& =\frac{1}{2} \log \frac{\left|\Sigma_2\right|}{\left|\Sigma_1\right|}-\frac{1}{2} E_{p(x)}\left[\left(x-\mu_1\right)^{\mathcal{T}} \Sigma_1^{-1}\left(x-\mu_1\right)\right]+\frac{1}{2} E_{p(x)}\left[\left(x-\mu_2\right)^{\mathcal{T}} \Sigma_2^{-1}\left(x-\mu_2\right)\right] \\
& =\frac{1}{2} \log \frac{\left|\Sigma_2\right|}{\left|\Sigma_1\right|}-\frac{1}{2}\left[\operatorname{tr}\left(\Sigma_1^{-1} \Sigma_1\right)+\left(\mu_1-\mu_1\right)^{\mathcal{T}} \Sigma_1^{-1}\left(\mu_1-\mu_1\right)\right]\\
&+\frac{1}{2}\left[\operatorname{tr}\left(\Sigma_2^{-1} \Sigma_1\right)+\left(\mu_1-\mu_2\right)^{\mathcal{T}} \Sigma_2^{-1}\left(\mu_1-\mu_2\right)\right] \\
& =\frac{1}{2} \log \frac{\left|\Sigma_2\right|}{\left|\Sigma_1\right|}-\frac{d}{2}+\frac{1}{2}\left[\operatorname{tr}\left(\Sigma_2^{-1} \Sigma_1\right)+\left(\mu_1-\mu_2\right)^{\mathcal{T}} \Sigma_2^{-1}\left(\mu_1-\mu_2\right)\right] \\
& =\frac{1}{2}\left[\log \frac{\left|\Sigma_2\right|}{\left|\Sigma_1\right|}-d+\operatorname{tr}\left(\Sigma_2^{-1} \Sigma_1\right)+\left(\mu_1-\mu_2\right)^{\mathcal{T}} \Sigma_2^{-1}\left(\mu_1-\mu_2\right)\right]
\end{aligned}
$$

\section{Setting of Hyper-parameters in Loss Function}
In Eq.~\ref{loss_all}, combining unified knowledge from different network layers, and the original training loss leads to a higher number of hyperparameters. Nonetheless, our method demonstrates minimal sensitivity to these parameters, as similar sets effectively serve various teacher-student pairings within the same dataset. Specifically, for the CIFAR-100 dataset, the parameters for $\alpha$, $\beta$ are set at 0.1, 0.1, respectively. Similarly, for ImageNet, these parameters are 1, 1, while for the COCO dataset, they are 1 and 1, respectively.

\section{ViTs Knowledge Distillation}
To further illustrate the universality of our approach, we conducted comparative experiments within the increasingly popular and high-performing Vision Transformers (ViTs) framework.
% %
ViTs are renowned for achieving superior results via stacked multi-head self-attention modules and additional components. Nonetheless, the significant computational costs associated with this method are noteworthy. As a result, the distillation of ViTs demands substantial consideration.
Table \ref{s_vit} demonstrates that our method can effectively transfer the knowledge from the teacher to the student, even in larger-scale ViTs models.
\begin{table}[h]
\vspace{-0.3cm}
\centering
\caption{Results of distilling ViTs on ImageNet-1K.}\label{s_vit}
\begin{tabular}{l|cc} 
\toprule
Teacher & \multicolumn{1}{c}{DeiT-small} & \multicolumn{1}{c}{DeiT III-Small}  \\
        & 80.69                          & 82.76                               \\
Student & \multicolumn{1}{c}{DeiT-Tiny}  & \multicolumn{1}{c}{DeiT-Tiny}       \\
        & 74.42                          & 74.42                               \\ 
\midrule
KD      
& 75.01                          & 76.01                               \\
NKD     
& 75.48                          & 76.68                               \\
ViTKD   
& 76.18                          & 77.78                               \\
Ours    & \textbf{76.42}        & \textbf{78.01}                       \\
\bottomrule
\end{tabular}
\vspace{-0.3cm}
\end{table}
% \section{Comparison with self-distillation}
% Self-distillation is a concept in deep learning that involves the use of non-uniform soft supervision to enhance its performance. Unlike other methods, self-distillation doesn’t require any external sources or extra computational cost to improve its performance. This unique characteristic makes it quite efficient.
% Table \ref{s_skd} demonstrates that, even in the absence of a teacher model, UniKD maintains effectiveness by imposing more comprehensive constraints from various layers, thereby ensuring that the network acquires valuable knowledge from diverse perspectives at different stages.
% \input{table/s_skd}
